# Supplementary material for: StreamForest: Efficient Online Video Understanding with Persistent Event Memory
Source: arXiv:2509.24871 source file (2025-09-29)
Supplement: Supplementary file 1 [file appendix.tex]

\pdfoutput=1
\pdfminorversion=7

\documentclass{article}

% if you need to pass options to natbib, use, e.g.:
\PassOptionsToPackage{numbers, compress}{natbib}
% before loading neurips_2025

% ready for submission
\usepackage{neurips_2025}
% \usepackage[preprint]{neurips_2025}
% to compile a preprint version, e.g., for submission to arXiv, add add the
% [preprint] option:

% to compile a camera-ready version, add the [final] option, e.g.:
    % \usepackage[final]{neurips_2025}

% to avoid loading the natbib package, add option nonatbib:
   % \usepackage[nonatbib]{neurips_2025}

\usepackage[utf8]{inputenc} % allow utf-8 input
\usepackage[T1]{fontenc}    % use 8-bit T1 fonts
\usepackage{hyperref}       % hyperlinks
\usepackage{url}            % simple URL typesetting
\usepackage{booktabs}       % professional-quality tables
\usepackage{amsfonts}       % blackboard math symbols
\usepackage{nicefrac}       % compact symbols for 1/2, etc.
\usepackage{microtype}      % microtypography
\usepackage{xcolor}         % colors

\usepackage{amsmath}
\usepackage{multirow}
\usepackage{tikz}
\usepackage{color}
\usepackage{pifont}
\usepackage{amssymb}
\usepackage{enumitem}
\usepackage{xspace}

\usepackage{graphicx}
\usepackage{caption} 
\usepackage{subcaption}
\usepackage{wrapfig}
\captionsetup[table]{skip=3pt}

 % for example
 % in other words

% \def\etal{\emph{et al}\onedot}
%
% --- inline annotations
%

% --- disable by uncommenting  
% \renewcommand{\TODO}[1]{}
% \renewcommand{\todo}[1]{#1}

\usepackage{graphicx}
\usepackage{amsmath}
\usepackage{amssymb}
\usepackage{booktabs}
\usepackage{adjustbox}
\usepackage{multirow}
\usepackage{arydshln}
\usepackage{colortbl}
\usepackage{amsfonts}       % blackboard math symbols
\usepackage{nicefrac}       % compact symbols for 1/2, etc.
\usepackage{microtype}      % microtypography
\usepackage{times}
\usepackage{epsfig}
\usepackage{tipa}
\usepackage[T1, OT1]{fontenc}
\DeclareTextSymbolDefault{\dh}{T1}
\usepackage{booktabs}
\usepackage{multirow}
\usepackage{color, colortbl}
\usepackage{pifont}
\usepackage{makecell}
\usepackage{threeparttable}
\usepackage{xcolor}
\usepackage{scalerel}
\usepackage{makecell}
\usepackage{tabu}
\usepackage{tikz}
\usepackage{marvosym}
\usepackage{xcolor} 

\definecolor{Gray}{gray}{0.5}
\definecolor{LGray}{gray}{0.9}
\definecolor{darkblue}{RGB}{94,110,186}
\definecolor{darkGreen}{RGB}{92, 148, 110}
\definecolor{myblue}{RGB}{14, 121, 178}
\definecolor{rightpath}{RGB}{248, 203, 173}
\definecolor{wrongpath}{RGB}{89, 89, 89}

\usepackage{tabulary}
\usepackage{tabulary,multirow,overpic,xcolor}
\newcolumntype{x}[1]{>{\centering\arraybackslash}m{#1pt}}
\newcolumntype{y}[1]{>{\arraybackslash}m{#1pt}}

\title{StreamForest: Efficient Online Video Understanding with Persistent Event Memory}

\begin{document}

\appendix
% Section 编号为 A, B, C ...
\renewcommand{\thesection}{\Alph{section}}
% Subsection 编号为 A.1, A.2 ...
\renewcommand{\thesubsection}{\Alph{section}.\arabic{subsection}}

\section*{Appendix}
\addcontentsline{toc}{section}{Appendix}

This appendix provides additional information to support the main text. Below is a table of contents for easy navigation:

\begin{itemize}
    \item \hyperref[app:sec:Details_of_OnlineIT]{\textbf{A}}~\textbf{Details of OnlineIT}
    \begin{itemize}
        \item \hyperref[app:sec:Details_of_OnlineIT:OnlineIT-general]{A.1}~OnlineIT-general
        \item \hyperref[app:sec:Details_of_OnlineIT:OnlineIT-drive]{A.2}~OnlineIT-drive
    \end{itemize}

    \item \hyperref[app:sec:Details_of_ODVBench]{\textbf{B}}~\textbf{Details of ODV-Bench}
    \begin{itemize}
        \item \hyperref[app:sec:Details_of_ODVBench:Task]{B.1}~Task Taxonomy and Formulation
        \item \hyperref[app:sec:Details_of_ODVBench:Statistics]{B.2}~Dataset Statistics
    \end{itemize}

    \item \hyperref[app:sec:More_Implementation_Details]{\textbf{C}}~\textbf{More Implementation Details}

    \item \hyperref[app:sec:Full_Performances]{\textbf{D}}~\textbf{Full Performances}
    \begin{itemize}
        \item \hyperref[app:sec:Full_Performances:StreamingBench]{D.1}~StreamingBench
        \item \hyperref[app:sec:Full_Performances:OVBench]{D.2}~OVBench
        \item \hyperref[app:sec:Full_Performances:OVO-Bench]{D.3}~OVO-Bench
    \end{itemize}

    \item \hyperref[app:sec:Qualitative_Comparison]{\textbf{E}}~\textbf{Qualitative Comparison}

    \item \hyperref[app:sec:More_Ablations]{\textbf{F}}~\textbf{More Ablations}

    \item \hyperref[app:sec:Discussions]{\textbf{G}}~\textbf{Discussions}
    \begin{itemize}
        \item \hyperref[app:sec:Discussions:Limitations]{G.1}~Limitations
        \item \hyperref[app:sec:Discussions:Broader Impacts]{G.2}~Broader Impacts
    \end{itemize}
\end{itemize}

\newpage

\input{paragraphs/7_Appendix}

\clearpage
{
\small
\bibliographystyle{plainnat}
\bibliography{reference}
}

\end{document}
